# Supplementary material for: Long-Context State-Space Video World Models
Source: arXiv:2505.20171 source file (2025-05-26)

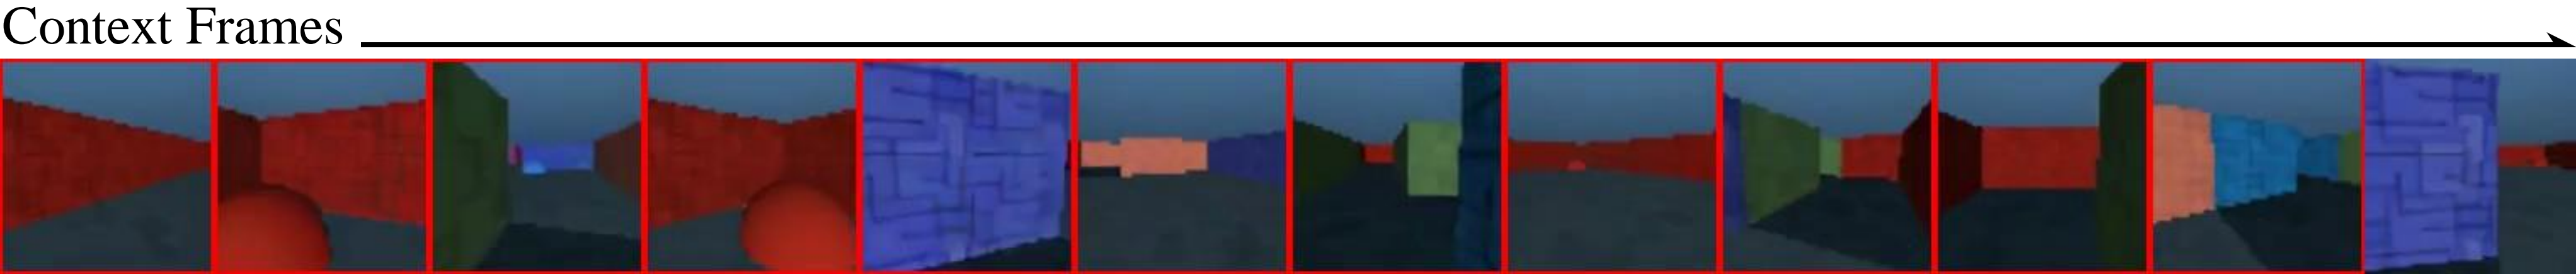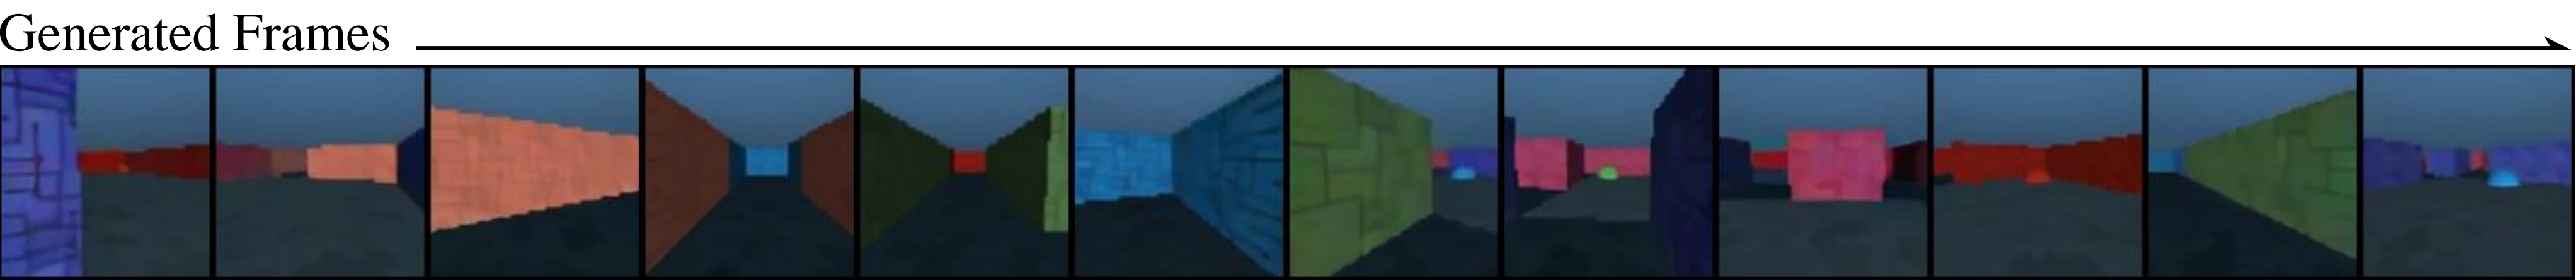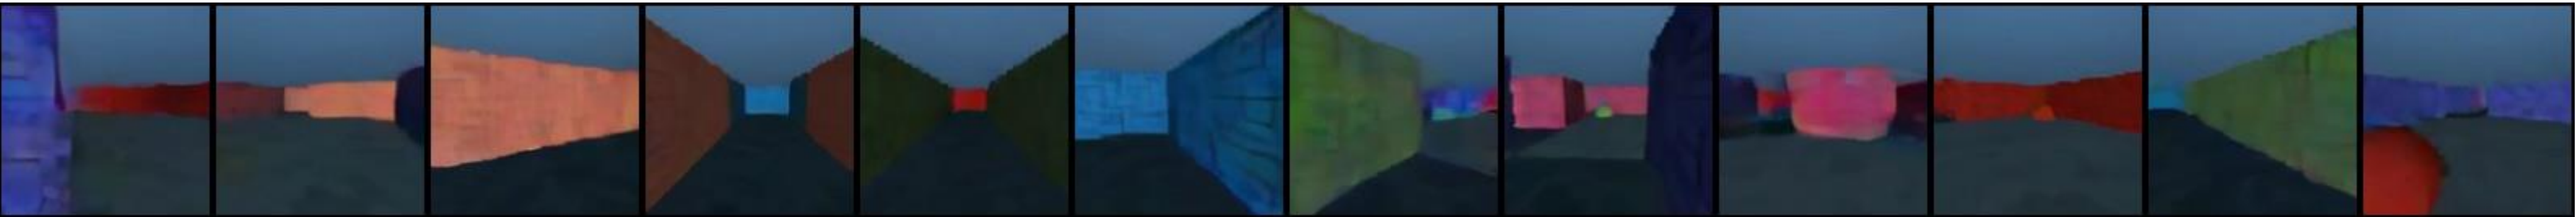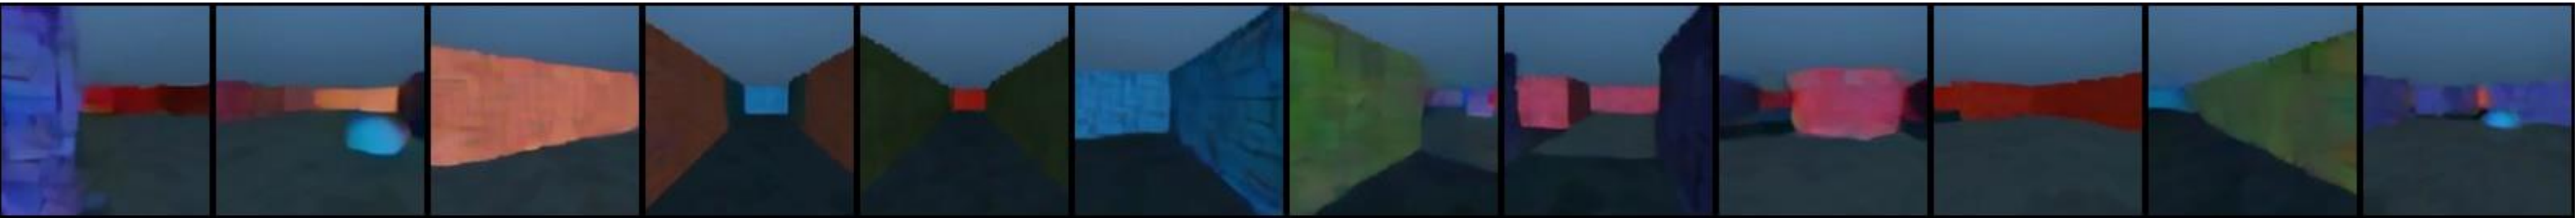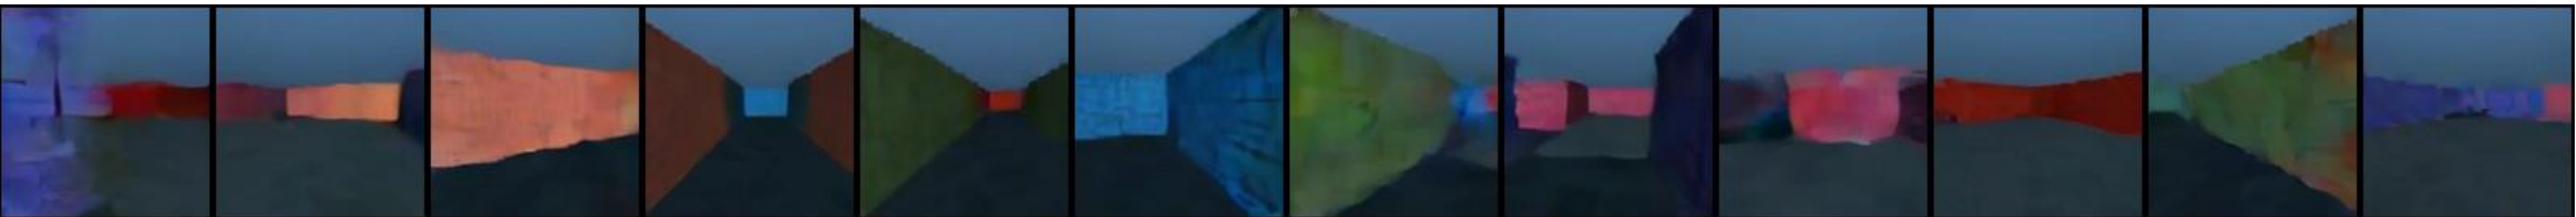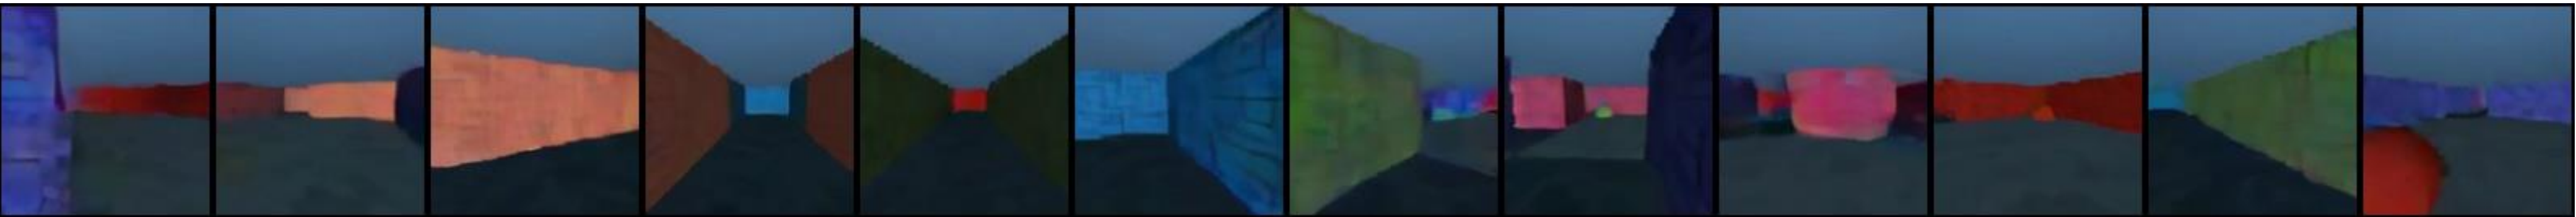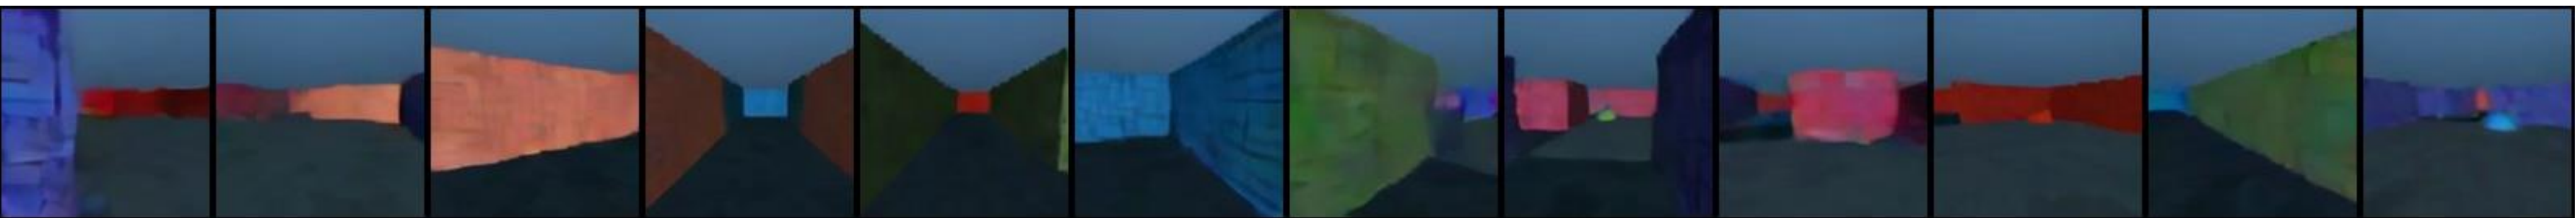



Context Frames

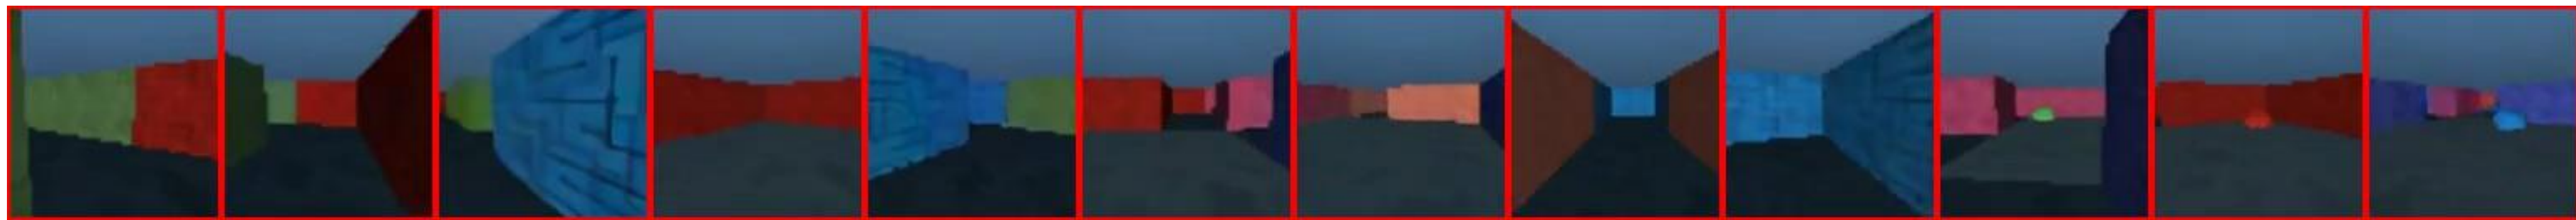

Generated Frames

GT

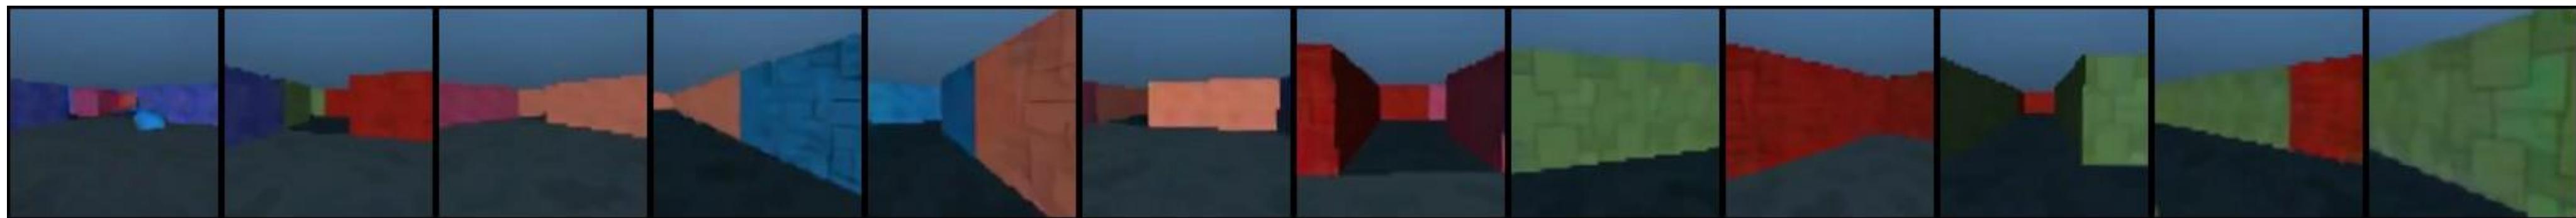

Ours

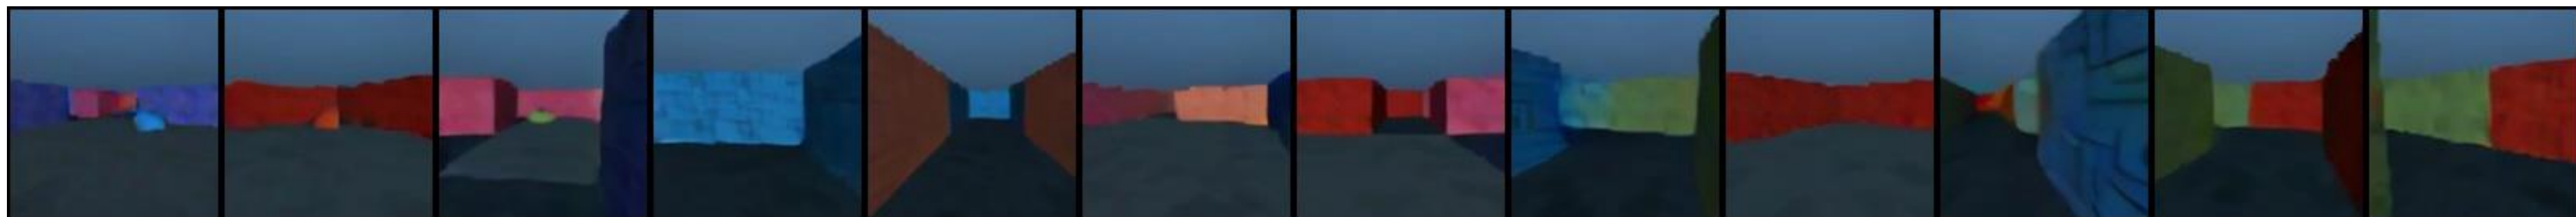

Causal  
(200 Context)

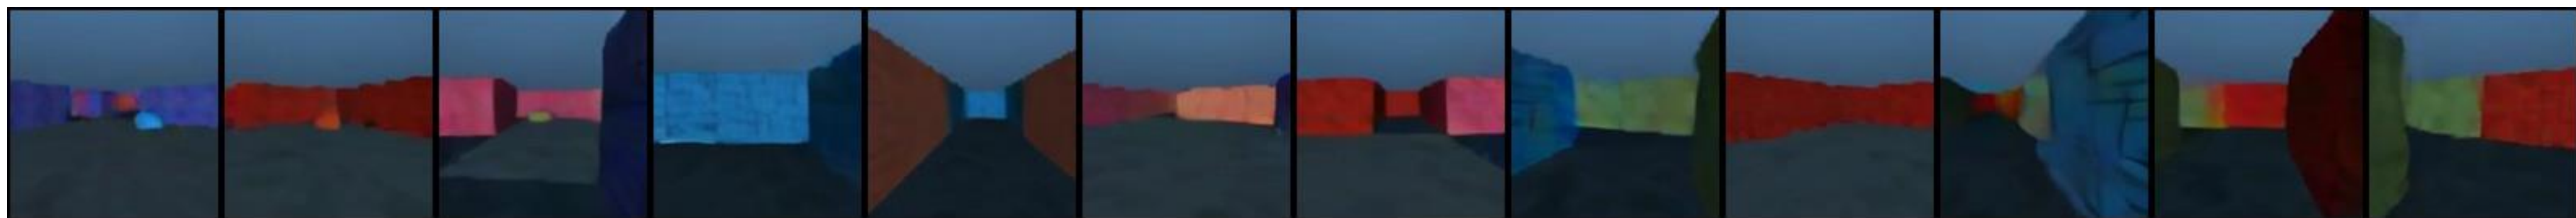

Mamba2

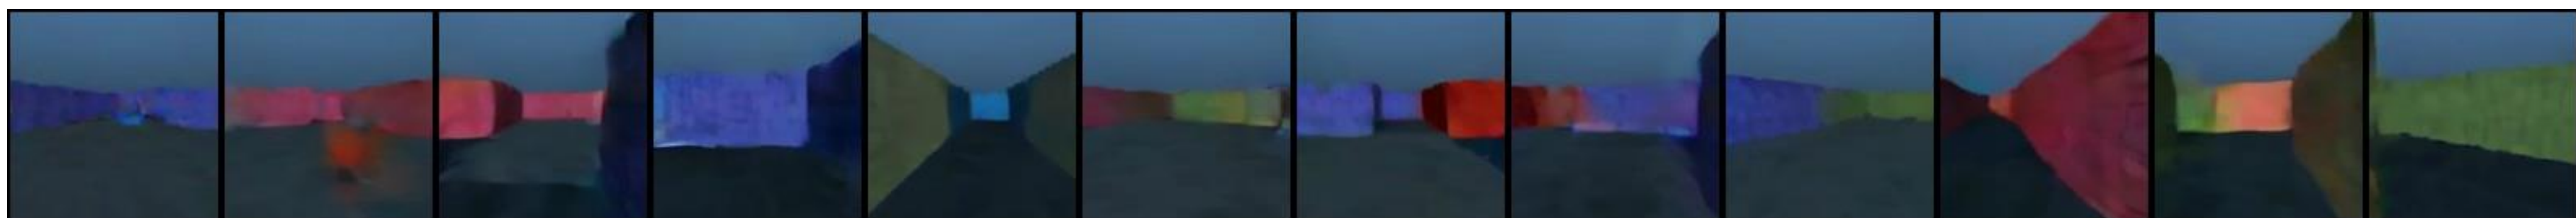

Mamba2 +  
Frame Local Attn

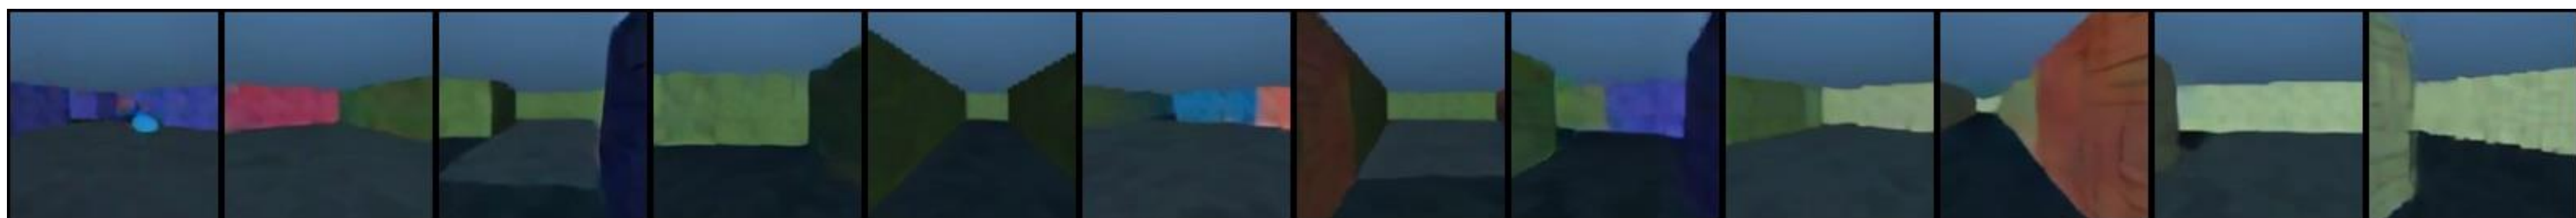

Causal  
(Full Context)

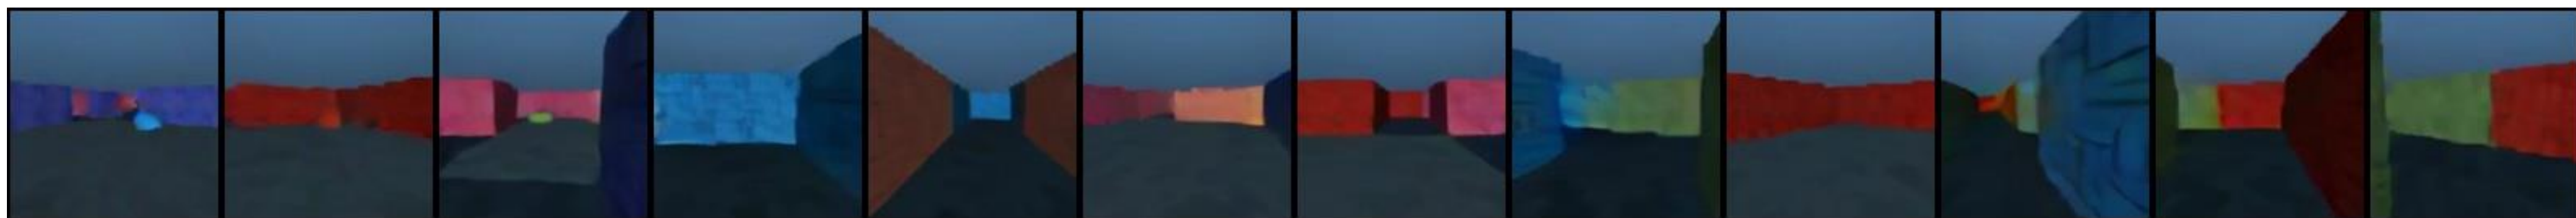

Supplement: Supplementary file 1 [file maze_supplement_reasoning.pdf]
